# Supplementary material for: Architecting Agentic Communities using Design Patterns
Source: arXiv:2601.03624 ancillary file (2026-05-25)
Supplement: Supplementary file 1 [file agentic-patterns-catalogue-v1.0.pdf]

# Complete Agentic AI Design Patterns Catalogue

---

## Pattern 1: ReAct (Reasoning and Acting)

**Agent Type:** Agentic AI

**What:** A pattern that interleaves reasoning traces with action execution, allowing the agent to think through problems step-by-step while taking actions and observing their outcomes.

**Why:** Enables more interpretable and robust decision-making by making the agent's reasoning process explicit and allowing it to adapt based on action results. The step-by-step reasoning with action execution demonstrates genuine agency through autonomous goal pursuit and dynamic decision-making.

**Mechanisms:** - Thought-action-observation cycles - Language model generates reasoning traces before each action - Actions can include tool use, information gathering, or environment manipulation - Observations from actions inform subsequent reasoning steps

**Agent Type Rationale:** ReAct embodies Agentic AI through its combination of autonomous reasoning and adaptive action-taking. The pattern demonstrates genuine agency by independently determining which actions to take based on observations and dynamically adjusting its approach based on results.

**Related Patterns:** - Uses: Tool-Using Agent (2), Memory-Augmented (3) - Used by: Hierarchical Planning (5), Orchestration (14) - Complements: Reflexion (6), Explanation (22), Metacognitive (11)

**References:** Yao et al. (2022) "ReAct: Synergizing Reasoning and Acting in Language Models"

## Pattern 2: Tool-Using Agent

**Agent Type:** AI Agent

**What:** An agent architecture that can dynamically select and use external tools (APIs, functions, software) to accomplish tasks beyond its base capabilities.

**Why:** Extends agent capabilities without retraining by leveraging existing tools and services, enabling more practical real-world applications. While powerful, this pattern typically serves as task-specific automation rather than demonstrating full autonomous agency.

**Mechanisms:** - Tool registry with descriptions and schemas - Tool selection logic (often learned or rule-based) - Parameter binding and execution handling - Error handling and retry mechanisms - Tool chaining for complex workflows

**Agent Type Rationale:** Tool-Using is classified as AI Agent because it primarily extends capabilities within a controlled scope. While it can dynamically select tools, it typically operates within predefined parameters and serves as a building block for more autonomous systems rather than exhibiting independent goal pursuit.

**Related Patterns:** - Used by: ReAct (1), Workflow (9), Orchestration (14) - Complements: Memory-Augmented (3) for learning tool usage patterns - Alternative to: Embodied Agent (10) for non-physical tasks

**References:** Schick et al. (2023) "Toolformer: Language Models Can Teach Themselves to Use Tools"

### Pattern 3: Memory-Augmented Agent

**Agent Type:** Agentic AI

**What:** An agent with persistent memory systems that can store, retrieve, and utilize information across interactions and sessions.

**Why:** Enables learning from experience, maintaining context over long periods, and building on previous interactions for better performance. The continuous learning and adaptation capabilities are hallmarks of genuine agency.

**Mechanisms:** - Short-term memory (working memory, conversation context) - Long-term memory (episodic, semantic, procedural knowledge) - Memory retrieval systems (vector databases, knowledge graphs) - Memory consolidation and forgetting mechanisms

**Agent Type Rationale:** Memory-Augmented represents Agentic AI through its self-learning capabilities. The pattern enables agents to learn from past experiences, adapt behavior over time, and pursue goals more effectively through accumulated knowledge—key characteristics of genuine agency.

**Related Patterns:** - Complements: ReAct (1), Reflexion (6), Metacognitive (11) - Enables: Adaptation/Personalization (30), Context Management (29) - Works with: Version Control (25) for memory versioning

**References:** Weng (2023) “LLM Powered Autonomous Agents”; Packer et al. (2023) “MemGPT”

### Pattern 4: Multi-Agent System (MAS)

**Agent Type:** Agentic System

**What:** Multiple autonomous agents that interact, coordinate, and potentially compete to achieve individual or collective goals.

**Why:** Enables division of labor, specialization, scalability, and emergent behaviors that single agents cannot achieve alone. The coordination framework represents system-level orchestration beyond individual agent capabilities.

**Mechanisms:** - Agent communication protocols (message passing, shared memory) - Coordination mechanisms (voting, consensus, market-based) - Role specialization and task allocation - Conflict resolution and negotiation protocols

**Agent Type Rationale:** Multi-Agent System is classified as Agentic System because it provides the coordination infrastructure for multiple agents to work together. The pattern focuses on system-level orchestration, emergent behaviors, and collective intelligence rather than individual agent capabilities.

**Related Patterns:** - Requires: Inter-Agent Communication (12) or simpler coordination - Often uses: Orchestration (14) for coordination - Can include: Ensemble (35) for robustness - May use: Negotiation (21) for complex agreements

**References:** Stone & Veloso (2000) “Multiagent Systems: A Survey”; Wu et al. (2023) “AutoGen”

### Pattern 5: Hierarchical Planning Agent

**Agent Type:** Agentic AI

**What:** An agent that decomposes complex, long-term goals into hierarchical subgoals and plans, operating at multiple levels of abstraction.

**Why:** Manages complexity of long-horizon tasks, enables more efficient planning, and provides natural points for human oversight and intervention. The autonomous goal decomposition and strategic planning demonstrate genuine agency.

**Mechanisms:** - Goal decomposition algorithms - Multi-level planning (strategic, tactical, operational) - Plan execution monitoring and replanning - Abstraction hierarchies for actions and states

**Agent Type Rationale:** Hierarchical Planning embodies Agentic AI through autonomous goal decomposition and strategic planning capabilities. The pattern demonstrates independent formulation of sub-goals and strategies to achieve higher-level objectives—a defining characteristic of genuine agency.

**Related Patterns:** - May use: ReAct (1) for plan execution - Related to: Decomposition (37) but more structured - Works with: Workflow (9) for execution - Complements: Metacognitive (11) for plan evaluation

**References:** Ahn et al. (2022) “Do As I Can, Not As I Say”; Huang et al. (2022) “Language Models as Zero-Shot Planners”

## **Pattern 6: Reflexion Agent**

**Agent Type:** Agentic AI

**What:** An agent that can self-reflect on its performance, learn from mistakes, and improve its behavior through iterative self-evaluation.

**Why:** Enables continuous improvement without external supervision, better error recovery, and adaptation to new situations. The self-improvement capability represents meta-agency—the highest form of autonomous learning.

**Mechanisms:** - Performance evaluation metrics and self-assessment - Failure analysis and error categorization - Strategy adjustment based on reflection - Experience replay and counterfactual reasoning

**Agent Type Rationale:** Reflexion represents Agentic AI through its meta-cognitive self-improvement capabilities. The pattern’s ability to reflect on its own performance and autonomously adjust strategies demonstrates the self-learning and continuous adaptation that defines genuine agency.

**Related Patterns:** - Builds on: ReAct (1) with added reflection layer - Works with: Memory-Augmented (3) to store learnings - Related to: Metacognitive (11), Feedback Loop (39) - Complements: Critic-Actor (8) for evaluation

**References:** Shinn et al. (2023) “Reflexion: Language Agents with Verbal Reinforcement Learning”

## **Pattern 7: Constitutional AI**

**Agent Type:** Agentic AI

**What:** An agent guided by a constitution (set of principles, values, rules) that shapes its behavior and decision-making.

**Why:** Ensures value alignment, safety, and ethical behavior without constant human oversight. The value-aligned autonomous behavior demonstrates controlled agency within ethical boundaries.

**Mechanisms:** - Constitutional principles defined upfront - Self-critique against constitutional principles - Revision process to align with principles - Reinforcement learning from constitution

**Agent Type Rationale:** Constitutional AI represents Agentic AI because it enables autonomous decision-making within value-aligned boundaries. The agent independently pursues goals while adhering to constitutional principles—demonstrating genuine agency constrained by ethical guidelines.

**Related Patterns:** - Works with: Compliance/Governance (18) for enforcement - Complements: Critic-Actor (8) for evaluation against constitution - Related to: Composable DSLs (44) for formal policy specification

**References:** Bai et al. (2022) “Constitutional AI: Harmlessness from AI Feedback”

## **Pattern 8: Critic-Actor**

**Agent Type:** Agentic AI

**What:** Separates the generation of outputs (actor) from their evaluation (critic), allowing for iterative refinement.

**Why:** Improves output quality through structured self-evaluation, enables better error detection, and provides natural points for explanation. The self-evaluation and refinement demonstrate cognitive agency.

**Mechanisms:** - Actor module generates candidates - Critic module evaluates quality - Iterative refinement loops - Feedback integration

**Agent Type Rationale:** Critic-Actor embodies Agentic AI through its combination of generation and autonomous evaluation capabilities. The pattern’s ability to self-assess and iteratively improve outputs demonstrates the cognitive agency required for sophisticated reasoning.

**Related Patterns:** - Used by: Reflexion (6), Progressive Refinement (24) - Complements: Constitutional AI (7) for value-aligned evaluation - Works with: Explanation (22) for transparency

**References:** Standard AI architecture pattern; widely used in RL and agent systems

## **Pattern 9: Workflow Agent**

**Agent Type:** Agentic AI

**What:** An agent that executes structured, multi-step workflows with branching logic, error handling, and state management.

**Why:** Manages complex business processes, ensures consistent execution, and provides auditability. The dynamic workflow execution with decision-making demonstrates operational agency.

**Mechanisms:** - Workflow definition and parsing - State machine execution - Branching logic and conditionals - Error handling and recovery - Progress tracking

**Agent Type Rationale:** Workflow Agent represents Agentic AI through its dynamic decision-making during workflow execution. While following structured processes, the agent makes contextual judgments about branching, error handling, and adaptation—demonstrating genuine agency within workflow constraints.

**Related Patterns:** - Uses: Tool-Using (2) for workflow steps - Related to: Hierarchical Planning (5) for complex workflows - May use: Human-in-the-Loop (40) for approvals - Complements: Orchestration (14) for multi-agent workflows

**References:** Standard enterprise pattern; adapted for LLM agents

### **Pattern 10: Embodied Agent**

**Agent Type:** Agentic AI

**What:** An agent that interacts with physical or simulated environments, perceiving and acting through sensors and actuators.

**Why:** Enables real-world interaction, grounds abstract reasoning in physical reality, and allows learning from environmental feedback. Physical environment interaction inherently requires genuine agency.

**Mechanisms:** - Sensor input processing - Action selection and execution - Environment state modeling - Feedback loop from actions to observations

**Agent Type Rationale:** Embodied Agent represents Agentic AI because physical or spatial environment interaction requires genuine autonomous decision-making. The agent must perceive, reason, plan, and act based on environmental context—demonstrating the full spectrum of agency.

**Related Patterns:** - Alternative to: Tool-Using (2) for physical tasks - May use: ReAct (1) for reasoning about actions - Works with: Memory-Augmented (3) for spatial memory

**References:** Robotics and embodied AI literature; Ahn et al. (2022) “Do As I Can, Not As I Say”

### **Pattern 11: Metacognitive Agent**

**Agent Type:** Agentic AI

**What:** An agent that can reason about its own cognitive processes, monitoring and controlling how it thinks, plans, and acts.

**Why:** Enables higher-order reasoning, better strategy selection, and adaptive problem-solving. Reasoning about reasoning represents the highest form of agency.

**Mechanisms:** - Self-monitoring of reasoning processes - Strategy evaluation and selection - Meta-level planning - Cognitive resource allocation

**Agent Type Rationale:** Metacognitive Agent embodies the highest form of Agentic AI through reasoning about its own thinking processes. This meta-level agency—the ability to monitor, evaluate, and adjust cognitive strategies—represents sophisticated autonomous intelligence.

**Related Patterns:** - Builds on: ReAct (1), Reflexion (6), Memory-Augmented (3) - Related to: Hierarchical Planning (5) for meta-level planning - Complements: Explanation (22) for reasoning transparency

**References:** Cox & Raja (2011) “Metareasoning”; emerging in LLM agents

### **Pattern 12: Inter-Agent Communication**

**Agent Type:** Agentic System

**What:** Structured protocols for agent-to-agent interaction with formal communication acts, accountability tracking, and deontic tokens (obligations, permissions, prohibitions).

**Why:** Enables rich multi-agent coordination with clear responsibility chains, supports compliance and auditability, and prevents communication breakdowns. System-level accountability infrastructure transcends individual agents.

**Mechanisms:** - Formal communication protocols (request, inform, commit, refuse) - Deontic tokens for obligations/permissions/prohibitions - Accountability chain tracking - Speech act theory implementation - Message queuing and routing

**Agent Type Rationale:** Inter-Agent Communication is classified as Agentic System because it provides system-level infrastructure for multi-agent coordination. The pattern focuses on formal protocols and accountability frameworks that enable agents to work together effectively—representing coordination beyond individual agent capabilities.

**Related Patterns:** - Required by: Multi-Agent System (4), Negotiation (21) - Uses: Semantic Bridge (15) for terminology translation - Works with: Audit Trail (20) for accountability - Related to: Composable DSLs (44) for formal policy specification

**References:** FIPA Agent Communication Language; ISO ODP Enterprise Language; Colombetti (2000) on commitment-based protocols

### Pattern 13: Human-Agent Communication

**Agent Type:** Agentic AI

**What:** Natural language interaction patterns between humans and agents, supporting clarification, negotiation, and mixed-initiative dialogue.

**Why:** Enables effective collaboration between humans and agents, supports iterative refinement of requirements, and provides transparency. Natural interaction requires contextual understanding and agency.

**Mechanisms:** - Natural language understanding and generation - Dialogue state tracking - Intent recognition and clarification - Mixed-initiative interaction - Context maintenance

**Agent Type Rationale:** Human-Agent Communication represents Agentic AI because effective human interaction requires contextual understanding, judgment, and adaptability. The agent must independently interpret intent, ask clarifying questions, and adjust communication style—demonstrating genuine agency in interaction.

**Related Patterns:** - Used by: Most user-facing patterns - Works with: Explanation (22) for transparency - May use: Human-in-the-Loop (40) for collaboration - Complements: Context Management (29) for dialogue history

**References:** Dialogue systems and conversational AI literature; mixed-initiative interaction research

### Pattern 14: Orchestration Agent

**Agent Type:** Agentic System

**What:** A coordinating agent that manages the lifecycle of multiple specialized agents, routing tasks, aggregating results, and handling inter-agent dependencies in complex workflows.

**Why:** Complex problems often require multiple specialized agents working together. Without orchestration, coordination becomes chaotic, error-prone, and difficult to monitor. The orchestration pattern provides centralized coordination while allowing individual agents to maintain their specialized capabilities. This system-level coordination represents the infrastructure needed for emergent multi-agent intelligence.

**Mechanisms:** - Task routing and agent selection based on capabilities - Workflow state management across multiple agents - Result aggregation and synthesis from multiple sources - Dependency tracking and execution ordering - Error handling and retry logic at the workflow level - Resource allocation and load balancing - Performance monitoring and optimization

**Agent Type Rationale:** Orchestration is classified as Agentic System because it provides the coordination infrastructure that enables multiple agents to work together effectively. The pattern focuses on system-level management rather than individual agent autonomy, creating the framework within which specialized agents can collaborate.

**Related Patterns:** - Manages: Multi-Agent System (4) workflows - Uses: Inter-Agent Communication (12) for coordination - Works with: Hierarchical Planning (5) for complex tasks - Complements: Workflow Agent (9) for structured processes - May use: Blackboard (42) for shared state

**References:** Wu et al. (2023) “AutoGen”; standard enterprise orchestration patterns adapted for AI agents

## Pattern 15: Semantic Bridge

**Agent Type:** Agentic System

**What:** An agent that translates between different domain terminologies, ontologies, and knowledge representations, enabling agents from different domains to communicate effectively.

**Why:** In multi-domain systems (e.g., healthcare integrating clinical, insurance, and research domains), agents use different vocabularies and conceptual frameworks. Without semantic translation, miscommunication leads to errors. The semantic bridge enables cross-domain agent collaboration by providing system-level semantic interoperability.

**Mechanisms:** - Ontology mapping and alignment - Terminology translation using domain dictionaries - Context-aware semantic interpretation - Concept normalization across domains - Ambiguity resolution through context - Standards-based translation (FHIR, SNOMED, ICD codes) - Bidirectional translation with validation

**Agent Type Rationale:** Semantic Bridge is classified as Agentic System because it enables system-wide communication across heterogeneous agents. The pattern provides infrastructure for semantic interoperability rather than individual agent capabilities, making it a coordination-level pattern.

**Related Patterns:** - Enables: Multi-Agent System (4) cross-domain collaboration - Works with: Inter-Agent Communication (12) for protocol alignment - Complements: Data Transformation (23) for syntax translation - Used by: Orchestration (14) for routing between domains

**References:** Ontology alignment literature; HL7 FHIR terminology services; semantic web research

## Pattern 16: Filtering/Triage Agent

**Agent Type:** AI Agent

**What:** An agent that performs preliminary filtering and prioritization of inputs, reducing information overload by selecting the most relevant items for downstream processing.

**Why:** Many applications face overwhelming input volumes that would be expensive or impossible to process completely. Early-stage filtering dramatically reduces computational costs while maintaining quality. This pattern provides task-specific automation within well-defined parameters.

**Mechanisms:** - Vector embeddings for semantic similarity - Threshold-based filtering using relevance scores - Multi-stage filtering pipelines (coarse to fine) - Priority queue management - Diversity-aware sampling to avoid information bubbles - Dynamic threshold adjustment based on load

**Agent Type Rationale:** Filtering/Triage is classified as AI Agent because it performs a specific, well-scoped automation task. While it may use sophisticated techniques like embeddings, it operates within predefined parameters without independent goal formulation, serving as a building block in larger systems.

**Related Patterns:** - Precedes: Structured Extraction (17), Validation (27) - Works with: Batch Processing (33) for volume handling - Complements: Context Management (29) for relevance - Used in: Data Processing Pipeline cluster

**References:** Information retrieval literature; clinical trial matching systems using embedding-based filtering

## **Pattern 17: Structured Extraction Agent**

**Agent Type:** AI Agent

**What:** An agent that converts unstructured or semi-structured data into structured, machine-readable formats suitable for downstream processing and analysis.

**Why:** Most real-world data exists in unstructured formats (text, PDFs, images). Converting to structured representations enables systematic processing, validation, and integration. This pattern provides essential data transformation capabilities as a building block for more complex systems.

**Mechanisms:** - Named entity recognition (NER) for key information - Relation extraction between entities - Schema-driven extraction with templates - LLM-based extraction with structured prompting - Validation against target schemas - Confidence scoring for extracted elements - Human-in-the-loop for ambiguous cases

**Agent Type Rationale:** Structured Extraction is classified as AI Agent because it performs a specific data transformation task within controlled parameters. While sophisticated, it follows clear input-output mappings and serves as a utility component in larger pipelines rather than exhibiting autonomous goal pursuit.

**Related Patterns:** - Follows: Filtering/Triage (16) in pipelines - Precedes: Data Transformation (23), Validation (27) - Works with: Tool-Using (2) for extraction tools - Complements: Semantic Bridge (15) for terminology - Used in: Clinical trial matching, document processing

**References:** NLP and information extraction literature; FHIR resource extraction; entity recognition research

## **Pattern 18: Compliance/Governance Agent**

**Agent Type:** Agentic System

**What:** A system-level agent that monitors and enforces regulatory requirements, organizational policies, and compliance constraints across multiple agents and workflows.

**Why:** Regulated industries (healthcare, finance, legal) require demonstrable compliance with complex regulations. System-level enforcement ensures all agents adhere to policies, creating audit trails and preventing violations. This pattern operates across the entire agent system rather than within individual agents.



**Mechanisms:** - Policy engine for rule evaluation - Real-time compliance monitoring - Violation detection and alerting - Automated policy enforcement gates - Compliance reporting and documentation - Integration with regulatory frameworks (HIPAA, SOC2, GDPR) - Dynamic policy updates without system downtime

**Agent Type Rationale:** Compliance/Governance is classified as Agentic System because it provides system-wide policy enforcement infrastructure. The pattern monitors and controls multiple agents, ensuring collective adherence to regulations—a coordination function that transcends individual agent capabilities.

**Related Patterns:** - Works with: Constitutional AI (7) for value alignment - Requires: Audit Trail (20) for documentation - Uses: Access Control (19) for enforcement - Complements: Composable DSLs (44) for policy specification - Related to: Validation (27) but system-level

**References:** Regulatory compliance literature; enterprise governance frameworks; responsible AI guidelines

## **Pattern 19: Access Control Agent**

**Agent Type:** Agentic System

**What:** A system-level agent that manages permissions, authorization, and access rights across agents, resources, and operations, ensuring security and appropriate delegation.

**Why:** Multi-agent systems require fine-grained access control to protect sensitive resources, maintain security boundaries, and enable delegation while preserving accountability. System-level access management ensures consistent enforcement across all agents.

**Mechanisms:** - Role-based access control (RBAC) - Attribute-based access control (ABAC) - Permission delegation chains with accountability - Token-based authorization (permit tokens) - Dynamic permission evaluation - Principle of least privilege enforcement - Integration with identity providers (OAuth, SAML)

**Agent Type Rationale:** Access Control is classified as Agentic System because it provides system-wide security infrastructure. The pattern manages permissions across multiple agents and resources, creating the security framework within which agents operate—a coordination function beyond individual agent scope.

**Related Patterns:** - Required by: Compliance/Governance (18) - Works with: Audit Trail (20) for security logging - Uses: Inter-Agent Communication (12) for permit tokens - Complements: Constitutional AI (7) for policy-based access - Enables: Federated Privacy-Aware (46) for data protection

**References:** Security and access control literature; SMART on FHIR; OAuth 2.0; enterprise IAM systems

## **Pattern 20: Audit Trail Agent**

**Agent Type:** Agentic System

**What:** A system-level agent that maintains comprehensive, tamper-proof logs of all agent activities, decisions, and interactions, providing complete traceability and accountability.

**Why:** Enterprise and regulated applications require demonstrable accountability, debugging capabilities, and compliance documentation. Comprehensive audit trails enable post-hoc analysis, regulatory reporting, and incident investigation. This pattern provides system-wide observability infrastructure.

**Mechanisms:** - Structured event logging with timestamps - Provenance tracking for all decisions - Tamper-proof log storage (blockchain, immutable storage) - Accountability chain recording - Searchable log querying - Retention policy management - Integration with SIEM systems

**Agent Type Rationale:** Audit Trail is classified as Agentic System because it provides system-wide monitoring and logging infrastructure. The pattern tracks activities across all agents, creating the observability framework needed for system-level accountability—a coordination function transcending individual agents.

**Related Patterns:** - Required by: Compliance/Governance (18) - Works with: Access Control (19) for security logging - Uses: Inter-Agent Communication (12) for tracking interactions - Complements: Monitoring/Observability (28) for real-time tracking - Enables: Explanation (22) for decision reconstruction

**References:** Provenance tracking research; blockchain for audit trails; enterprise logging standards; regulatory compliance frameworks

## **Pattern 21: Negotiation Agent**

**Agent Type:** Agentic System

**What:** An agent that facilitates multi-party negotiation and agreement-reaching through structured proposal, counter-proposal, and consensus-building protocols.

**Why:** Complex decisions often require multiple stakeholders with different objectives to reach agreement. Structured negotiation enables distributed decision-making while preserving individual agent autonomy. This pattern provides the coordination infrastructure for multi-party agreements in agent systems.

**Mechanisms:** - Proposal generation and evaluation - Counter-proposal formulation - Concession strategies and compromise - Voting and consensus mechanisms - Conflict resolution protocols - Negotiation history tracking - Commitment enforcement

**Agent Type Rationale:** Negotiation is classified as Agentic System because it coordinates multiple autonomous agents to reach collective decisions. The pattern provides the infrastructure for multi-party coordination requiring sophisticated interaction protocols—a system-level coordination capability.

**Related Patterns:** - Specialized form of: Inter-Agent Communication (12) - Related to: Debate/Deliberation (43) but outcome-focused - Works with: Multi-Agent System (4) for coordination - May use: Constitutional AI (7) for negotiation principles - Complements: Orchestration (14) for workflow integration

**References:** Multi-agent negotiation literature; game theory; distributed AI systems; automated trading systems

## **Pattern 22: Explanation Agent**

**Agent Type:** Agentic AI

**What:** An agent that generates human-understandable explanations of decisions, reasoning processes, and behaviors, making AI systems interpretable and trustworthy.

**Why:** Users need to understand, trust, and potentially challenge AI decisions, especially in high-stakes domains. Effective explanations build trust, enable debugging, and support regulatory compliance. Generating quality explanations requires contextual understanding and judgment—characteristics of genuine agency.

**Mechanisms:** - Reasoning trace extraction and summarization - Counterfactual explanation generation - Feature importance visualization - Natural language explanation generation - Multi-level explanations (brief, detailed, technical) - Example-based explanations - Interactive explanation refinement

**Agent Type Rationale:** Explanation is classified as Agentic AI because generating effective explanations requires contextual reasoning about what information is relevant, how to present it clearly, and what level of detail is appropriate. This judgment and adaptation demonstrate genuine agency in communication.

**Related Patterns:** - Works with: ReAct (1) for reasoning traces - Complements: Human-Agent Communication (13) for delivery - Uses: Audit Trail (20) for decision provenance - Related to: Metacognitive (11) for self-awareness - Required by: Compliance/Governance (18) in regulated domains

**References:** Explainable AI (XAI) literature; LIME, SHAP; narrative generation research; human-computer interaction studies

### **Pattern 23: Data Transformation Agent**

**Agent Type:** AI Agent

**What:** An agent that converts data between different formats, schemas, and representations, enabling interoperability between systems with different data models.

**Why:** Systems often use incompatible data formats and schemas. Transformation enables integration without requiring all systems to adopt a single standard. This pattern provides essential ETL (Extract-Transform-Load) capabilities as a building block for data pipelines.

**Mechanisms:** - Schema mapping and translation - Format conversion (JSON, XML, CSV, etc.) - Data normalization and standardization - Type conversion and casting - Aggregation and disaggregation - Validation after transformation - Batch and streaming transformation modes

**Agent Type Rationale:** Data Transformation is classified as AI Agent because it performs specific, well-defined data conversion tasks within controlled parameters. While it may handle complex transformations, it operates with clear input-output mappings and serves as a utility component rather than exhibiting autonomous decision-making.

**Related Patterns:** - Follows: Structured Extraction (17) in pipelines - Works with: Semantic Bridge (15) for meaning preservation - Precedes: Validation (27) for quality checking - Complements: Batch Processing (33) for volume - Used in: Integration and data pipeline scenarios

**References:** ETL literature; data integration patterns; FHIR transformation services; enterprise integration patterns

### **Pattern 24: Progressive Refinement Agent**

**Agent Type:** Agentic AI

**What:** An agent that iteratively improves output quality through multiple refinement cycles, each building on previous results with increasingly sophisticated processing.

**Why:** Many tasks benefit from iterative improvement rather than single-pass generation. Progressive refinement enables quality-time trade-offs and incremental delivery. The pattern requires evaluation judgment and strategy adjustment—characteristics of genuine agency.

**Mechanisms:** - Multi-pass processing with increasing sophistication - Quality evaluation after each pass - Stopping criteria based on quality thresholds or time - Incremental result delivery - Refinement strategy selection - Resource allocation across passes - Convergence detection

**Agent Type Rationale:** Progressive Refinement is classified as Agentic AI because it requires autonomous evaluation of quality and dynamic adjustment of refinement strategies. The pattern demonstrates genuine agency through its ability to assess results and determine optimal refinement approaches.

**Related Patterns:** - Uses: Critic-Actor (8) for evaluation - Related to: Reflexion (6) but focused on output - Works with: Feedback Loop (39) for learning - Complements: Human-in-the-Loop (40) for approval gates - May use: Ensemble (35) for multi-approach refinement

**References:** Iterative refinement literature; self-critique in LLMs; progressive rendering in graphics

## **Pattern 25: Version Control Agent**

**Agent Type:** AI Agent

**What:** An agent that tracks changes to data, models, prompts, and configurations over time, enabling rollback, comparison, and audit of modifications.

**Why:** AI systems evolve through experimentation and updates. Version control enables safe experimentation, rollback of problematic changes, and understanding of system evolution. This pattern provides essential tracking capabilities as a utility function.

**Mechanisms:** - Version tagging and naming - Change tracking with diffs - Rollback capabilities - Branch and merge operations - Version comparison and analysis - Metadata tracking (who, when, why) - Integration with Git and similar systems

**Agent Type Rationale:** Version Control is classified as AI Agent because it performs a specific tracking and management task within well-defined parameters. While important, it operates as a utility function without independent goal formulation or adaptive decision-making.

**Related Patterns:** - Works with: Memory-Augmented (3) for history - Complements: Audit Trail (20) for accountability - Enables: Error Recovery (31) through rollback - Used by: Progressive Refinement (24) for tracking - Supports: Compliance/Governance (18) for change documentation

**References:** Version control systems (Git, SVN); MLOps and model versioning; configuration management patterns

## **Pattern 26: Summarization Agent**

**Agent Type:** AI Agent

**What:** An agent that condenses large volumes of information into concise summaries while preserving key points, enabling efficient information consumption.

**Why:** Information overload is a constant challenge. Effective summarization enables users to quickly understand essential content without reading everything in full. This pattern provides focused automation for a specific information processing task.

**Mechanisms:** - Extractive summarization (selecting key sentences) - Abstractive summarization (generating new text) - Multi-document summarization - Query-focused summarization - Length-controlled output - Key point identification and ranking - Factual consistency verification

**Agent Type Rationale:** Summarization is classified as AI Agent because it performs a specific, well-scoped information processing task. While it may use sophisticated language models, it operates within predefined parameters (input text â†’ summary) and serves as a utility component in information pipelines.

**Related Patterns:** - Used in: Data Processing Pipeline cluster - Works with: Filtering/Triage (16) for focus - Complements: Explanation (22) for clarity - May use: Validation (27) for quality - Precedes: Human-Agent Communication (13) for delivery

**References:** Summarization research literature; abstractive summarization with transformers; ROUGE metrics

## **Pattern 27: Validation Agent**

**Agent Type:** AI Agent

**What:** An agent that verifies correctness, quality, and compliance of data, outputs, or system states against defined criteria, schemas, or constraints.

**Why:** Quality assurance is essential in production systems. Automated validation catches errors early, prevents propagation of invalid data, and ensures outputs meet requirements. This pattern provides systematic quality checking as a building block.

**Mechanisms:** - Schema validation against formal specifications - Constraint checking (business rules, data integrity) - Format verification - Completeness checking - Cross-validation with reference data - Anomaly detection - Multi-level validation (syntax, semantics, pragmatics)

**Agent Type Rationale:** Validation is classified as AI Agent because it performs specific verification tasks within well-defined rules and parameters. While important for quality assurance, it operates with clear correctness criteria rather than exhibiting autonomous goal pursuit.

**Related Patterns:** - Used by: Most patterns for quality assurance - Follows: Data Transformation (23) in pipelines - Works with: Critic-Actor (8) for evaluation - Complements: Error Recovery (31) for handling failures - Required by: Compliance/Governance (18) for policy enforcement

**References:** Data validation patterns; schema validation (JSON Schema, XML Schema); constraint checking in databases

## **Pattern 28: Monitoring/Observability Agent**

**Agent Type:** AI Agent

**What:** An agent that collects metrics, tracks system behavior, detects anomalies, and provides alerts, enabling operational awareness and incident response.

**Why:** Production systems require continuous monitoring to detect issues, understand performance, and trigger interventions. Observability enables debugging, optimization, and reliability. This pattern provides essential operational infrastructure.

**Mechanisms:** - Metrics collection (latency, throughput, error rates) - Distributed tracing across agents - Anomaly detection and alerting - Dashboard and visualization - Log aggregation and analysis - Performance profiling - Health checking

**Agent Type Rationale:** Monitoring/Observability is classified as AI Agent because it performs specific metrics collection and tracking tasks. While it may use sophisticated anomaly detection, it operates within predefined monitoring parameters rather than exhibiting autonomous strategic decision-making.

**Related Patterns:** - Complements: Audit Trail (20) for detailed logging - Works with: Error Recovery (31) for incident response - Enables: Fallback/Graceful Degradation (32) through health awareness - Used by: Orchestration (14) for workflow monitoring - Supports: Performance Optimization patterns

**References:** Observability literature; OpenTelemetry; Prometheus; distributed tracing systems; SRE practices

## **Pattern 29: Context Management Agent**

**Agent Type:** Agentic AI

**What:** An agent that maintains and dynamically manages relevant context across interactions, ensuring appropriate information is available while respecting token limits and relevance.

**Why:** LLM-based agents face context window constraints but need relevant historical information. Effective context management balances completeness with conciseness, requiring judgment about relevance—a characteristic of genuine agency.

**Mechanisms:** - Relevance scoring for context items - Dynamic context window allocation - Summarization of older context - Hierarchical context (immediate, recent, distant) - Context compression techniques - Retrieval-augmented context injection - User-specific context personalization

**Agent Type Rationale:** Context Management is classified as Agentic AI because it requires dynamic decision-making about what information is relevant and how to best utilize limited context space. This contextual judgment and adaptive strategy demonstrates genuine agency in information management.

**Related Patterns:** - Essential for: Memory-Augmented (3) agents - Works with: Summarization (26) for compression - Complements: Human-Agent Communication (13) for dialogue - Used by: ReAct (1) for maintaining state - Related to: Caching/Memoization (36) for efficiency

**References:** Context window management literature; MemGPT; retrieval-augmented generation (RAG); dialogue state tracking

## **Pattern 30: Adaptation/Personalization Agent**

**Agent Type:** Agentic AI

**What:** An agent that learns user preferences, adapts behavior to individual users, and personalizes interactions based on accumulated knowledge of user characteristics.

**Why:** Different users have different needs, preferences, and communication styles. Personalization improves user experience and effectiveness. The continuous learning and adaptation to user preferences demonstrates genuine agency through self-improvement.

**Mechanisms:** - User modeling and profiling - Preference learning from interactions - Behavioral adaptation based on feedback - A/B testing for optimization - Personalized recommendation - Communication style adaptation - Progressive disclosure based on expertise level

**Agent Type Rationale:** Adaptation/Personalization is classified as Agentic AI because it demonstrates continuous learning from experience and autonomous adjustment of behavior. The pattern exhibits genuine agency through its ability to independently learn user preferences and adapt strategies accordingly.

**Related Patterns:** - Uses: Memory-Augmented (3) for user history - Works with: Feedback Loop (39) for learning - Complements: Human-Agent Communication (13) for interaction -

Related to: Reflexion (6) for self-improvement - May use: A/B testing and reinforcement learning

**References:** Personalization systems; recommendation engines; adaptive user interfaces; learning from human feedback

### **Pattern 31: Error Recovery Agent**

**Agent Type:** Agentic AI

**What:** An agent that detects errors, diagnoses failure causes, and implements recovery strategies to restore normal operation or achieve goals through alternative means.

**Why:** Errors are inevitable in complex systems. Intelligent recovery requires understanding what went wrong and selecting appropriate corrective actions—requiring judgment and problem-solving that characterize genuine agency.

**Mechanisms:** - Error detection and classification - Root cause analysis - Recovery strategy selection - Retry logic with backoff - Alternative approach identification - Partial result preservation - Graceful degradation when recovery fails

**Agent Type Rationale:** Error Recovery is classified as Agentic AI because it requires autonomous diagnosis of failures and intelligent selection of recovery strategies. The pattern demonstrates genuine agency through its ability to analyze situations and adaptively determine appropriate responses.

**Related Patterns:** - Works with: Fallback/Graceful Degradation (32) for alternatives - Uses: Validation (27) for error detection - Complements: Monitoring/Observability (28) for detection - Related to: Reflexion (6) for learning from errors - May trigger: Human-in-the-Loop (40) for escalation

**References:** Error handling patterns; circuit breaker pattern; retry policies; resilience engineering

### **Pattern 32: Fallback/Graceful Degradation Agent**

**Agent Type:** Agentic AI

**What:** An agent that provides degraded but useful service when full capabilities are unavailable, intelligently selecting appropriate fallback strategies based on context.

**Why:** Systems should remain useful even when components fail or resources are constrained. Intelligent degradation requires understanding priorities and selecting appropriate reduced functionality—requiring contextual judgment that demonstrates genuine agency.

**Mechanisms:** - Capability tiering (full, reduced, minimal) - Fallback chain with progressively simpler approaches - Context-aware strategy selection - Quality vs. speed trade-offs - Resource-constrained operation modes - User notification of degraded service - Automatic recovery when possible

**Agent Type Rationale:** Fallback/Graceful Degradation is classified as Agentic AI because selecting appropriate degradation strategies requires contextual judgment and priority assessment. The pattern demonstrates genuine agency through adaptive decision-making about acceptable quality-performance trade-offs.

**Related Patterns:** - Works with: Error Recovery (31) for failure handling - Uses: Monitoring/Observability (28) for capability awareness - Complements: Ensemble (35) for backup approaches - Related to: Caching/Memoization (36) for cached results - May trigger: Human-in-the-Loop (40) for approval

**References:** Resilience engineering; graceful degradation patterns; circuit breaker; bulkhead patterns

### **Pattern 33: Batch Processing Agent**

**Agent Type:** AI Agent

**What:** An agent that efficiently processes large volumes of similar tasks in batches, optimizing throughput through parallelization and resource management.

**Why:** Many scenarios involve processing thousands or millions of similar items. Batch processing dramatically improves efficiency compared to one-at-a-time processing. This pattern provides bulk processing capabilities as an optimization technique.

**Mechanisms:** - Batch collection and sizing - Parallel processing within batches - Resource pooling and reuse - Progress tracking and checkpointing - Error handling for batch items - Priority-based scheduling - Cost optimization through batching

**Agent Type Rationale:** Batch Processing is classified as AI Agent because it performs specific bulk processing optimization within well-defined parameters. While it improves efficiency, it operates as a utility function for volume handling rather than exhibiting autonomous goal pursuit.

**Related Patterns:** - Alternative to: Real-Time/Streaming (34) for non-time-sensitive tasks - Works with: Parallel Processing (38) for throughput - Complements: Caching/Memoization (36) for efficiency - Uses: Filtering/Triage (16) for volume reduction - Supports: Data processing pipelines

**References:** Batch processing patterns; MapReduce; ETL systems; parallel processing literature

### **Pattern 34: Real-Time/Streaming Agent**

**Agent Type:** Agentic AI

**What:** An agent that processes continuous data streams with low latency, making decisions and taking actions on streaming data in real-time.

**Why:** Many applications require immediate responses to incoming data (market data, sensor streams, user interactions). Real-time processing with adaptive decision-making demonstrates genuine agency through dynamic responsiveness to changing conditions.

**Mechanisms:** - Event stream processing - Windowing and aggregation over time - Low-latency decision-making - State management in streams - Back-pressure handling - Out-of-order event handling - Stream joins and enrichment

**Agent Type Rationale:** Real-Time/Streaming is classified as Agentic AI because processing streaming data requires dynamic decision-making and adaptive responses to changing conditions. The pattern demonstrates genuine agency through its ability to make autonomous, time-sensitive decisions based on streaming context.

**Related Patterns:** - Alternative to: Batch Processing (33) for time-sensitive tasks - Works with: Monitoring/Observability (28) for stream monitoring - May use: Caching/Memoization (36) for frequent queries - Complements: Error Recovery (31) for stream failures - Used in: Trading systems, IoT applications

**References:** Stream processing systems (Kafka, Flink, Spark Streaming); event-driven architectures; reactive systems



### Pattern 35: Ensemble Agent

**Agent Type:** Agentic System

**What:** A system that combines outputs from multiple agents or models through voting, averaging, or weighted aggregation to improve robustness and accuracy.

**Why:** Different agents have different strengths and weaknesses. Ensemble approaches achieve better results than individual agents by combining diverse perspectives. This pattern provides system-level robustness through multi-agent coordination.

**Mechanisms:** - Majority voting for classification tasks - Weighted averaging for regression - Confidence-based aggregation - Diverse agent selection strategies - Disagreement detection and resolution - Meta-learning for weight optimization - Dynamic ensemble composition

**Agent Type Rationale:** Ensemble is classified as Agentic System because it coordinates multiple agents to achieve collective intelligence. The pattern focuses on system-level combination strategies rather than individual agent capabilities, representing multi-agent coordination infrastructure.

**Related Patterns:** - Form of: Multi-Agent System (4) with aggregation focus - Works with: Debate/Deliberation (43) for disagreement resolution - Complements: Fallback/Graceful Degradation (32) for robustness - May use: Critic-Actor (8) for quality assessment - Related to: Negotiation (21) but output-focused

**References:** Ensemble learning literature; mixture of experts; multi-agent consensus; wisdom of crowds

### Pattern 36: Caching/Memoization Agent

**Agent Type:** AI Agent

**What:** An agent that stores previously computed results and retrieves them for identical or similar requests, improving performance by avoiding redundant computation.

**Why:** Many tasks involve repeated queries or similar inputs. Caching dramatically improves response time and reduces computational costs. This pattern provides essential performance optimization as a utility function.

**Mechanisms:** - Cache key generation from inputs - Storage backends (memory, Redis, databases) - Cache hit/miss handling - Eviction policies (LRU, LFU, TTL) - Similarity-based retrieval for near-matches - Cache warming and preloading - Distributed caching for scale

**Agent Type Rationale:** Caching/Memoization is classified as AI Agent because it performs specific performance optimization within well-defined parameters. While important for efficiency, it operates as a utility function without independent goal formulation or adaptive strategy.

**Related Patterns:** - Complements: Real-Time/Streaming (34) for low latency - Works with: Context Management (29) for retrieval - Used by: Most patterns for performance - Related to: Memory-Augmented (3) but focused on efficiency - Supports: Batch Processing (33) for throughput

**References:** Caching patterns; CDN architecture; database caching; Redis; memcached

### Pattern 37: Decomposition Agent

**Agent Type:** Agentic AI

**What:** An agent that breaks complex tasks into smaller, manageable subtasks, identifying dependencies and creating execution plans.

**Why:** Complex problems overwhelm single-step approaches. Decomposition enables parallelization, focused attention, and systematic problem-solving. Intelligent task breakdown requires understanding task structure and dependencies—demonstrating genuine agency.

**Mechanisms:** - Task analysis and breakdown - Dependency identification - Subtask sequencing and ordering - Complexity estimation - Recursive decomposition for nested problems - Work breakdown structure creation - Dynamic decomposition based on progress

**Agent Type Rationale:** Decomposition is classified as Agentic AI because breaking down complex tasks requires autonomous analysis and strategic planning. The pattern demonstrates genuine agency through its ability to independently assess task structure and formulate decomposition strategies.

**Related Patterns:** - Related to: Hierarchical Planning (5) but task-focused - Used by: Orchestration (14) for workflow creation - Works with: Parallel Processing (38) for concurrent execution - Complements: Plan-then-Execute (41) for planning - Enables: Multi-Agent System (4) task allocation

**References:** Task decomposition literature; work breakdown structures; problem decomposition in planning

### **Pattern 38: Parallel Processing Agent**

**Agent Type:** AI Agent

**What:** An agent that executes independent tasks simultaneously across multiple threads, processes, or machines to improve throughput and reduce latency.

**Why:** Many tasks can be performed concurrently without dependencies. Parallelization dramatically improves performance on multi-core systems. This pattern provides essential concurrency management as a utility function.

**Mechanisms:** - Task independence analysis - Thread pool management - Process spawning and coordination - Distributed task execution - Result aggregation from parallel tasks - Load balancing across workers - Error isolation between parallel tasks

**Agent Type Rationale:** Parallel Processing is classified as AI Agent because it performs specific concurrency management within well-defined parameters. While it improves performance, it operates as infrastructure for concurrent execution rather than exhibiting autonomous strategic decision-making.

**Related Patterns:** - Works with: Batch Processing (33) for volume - Enables: Decomposition (37) task execution - Complements: Orchestration (14) for coordination - Used by: Ensemble (35) for parallel inference - Supports: Real-Time/Streaming (34) for throughput

**References:** Parallel computing patterns; MapReduce; concurrent programming; distributed systems

### **Pattern 39: Feedback Loop Agent**

**Agent Type:** Agentic AI

**What:** An agent that collects feedback on its outputs and actions, analyzes feedback to identify improvement opportunities, and adjusts behavior accordingly.

**Why:** Continuous improvement requires learning from experience. Feedback loops enable agents to evolve and improve over time without explicit reprogramming. The autonomous incorporation of feedback demonstrates genuine agency through self-directed learning.

**Mechanisms:** - Feedback collection (explicit, implicit, automated) - Feedback analysis and pattern identification - Performance metric tracking - Behavior adjustment strategies - A/B testing for improvement validation - Feedback integration into models - Long-term learning and evolution

**Agent Type Rationale:** Feedback Loop is classified as Agentic AI because incorporating feedback requires autonomous evaluation and adaptive strategy adjustment. The pattern demonstrates genuine agency through its ability to learn from experience and independently improve performance.

**Related Patterns:** - Similar to: Reflexion (6) but feedback-focused - Works with: Memory-Augmented (3) for learning storage - Complements: Adaptation/Personalization (30) for improvement - Uses: Monitoring/Observability (28) for metrics - Related to: Human-in-the-Loop (40) for human feedback

**References:** Reinforcement learning; online learning; feedback-driven improvement; human-in-the-loop learning

#### **Pattern 40: Human-in-the-Loop Agent**

**Agent Type:** Agentic AI

**What:** An agent that integrates human judgment at critical decision points, escalating to humans when confidence is low, stakes are high, or errors would be costly.

**Why:** Full automation isn't always appropriate. Human oversight provides safety, handles edge cases, and builds trust. Knowing when to escalate requires judgment about uncertainty and stakes—demonstrating genuine agency in collaboration.

**Mechanisms:** - Confidence-based escalation triggers - Human interface for review and intervention - Feedback collection from human decisions - Learning from human corrections - Asynchronous human input handling - Priority-based human queue management - Progressive automation as confidence grows

**Agent Type Rationale:** Human-in-the-Loop is classified as Agentic AI because determining when to involve humans requires autonomous assessment of confidence and risk. The pattern demonstrates genuine agency through intelligent collaboration with humans rather than pure automation.

**Related Patterns:** - Works with: Explanation (22) for decision transparency - Complements: Plan-then-Execute (41) for approval gates - Uses: Human-Agent Communication (13) for interaction - Related to: Error Recovery (31) for escalation - Supports: Compliance/Governance (18) for oversight

**References:** Human-in-the-loop machine learning; active learning; human-AI collaboration research; mixed-initiative systems

#### **Pattern 41: Plan-then-Execute Agent**

**Agent Type:** Agentic AI

**What:** An agent that separates planning from execution, generating an explicit, auditable plan that can be reviewed (often by humans) before any side-effecting actions are taken.

**Why:** Many high-stakes scenarios require transparency and oversight before action. Separating planning from execution enables review, rollback planning, and safer operation. The strategic separation of planning and execution demonstrates sophisticated agency.

**Mechanisms:** - Explicit plan generation phase - Plan representation in structured format - Human approval gates before execution - Plan validation and feasibility checking - Execution monitoring against plan - Plan revision based on execution feedback - Rollback capabilities using plan structure

**Agent Type Rationale:** Plan-then-Execute is classified as Agentic AI because generating comprehensive plans and managing the planning-execution lifecycle requires autonomous strategic reasoning. The pattern demonstrates genuine agency through sophisticated multi-phase goal pursuit with built-in oversight mechanisms.

**Related Patterns:** - Alternative to: ReAct (1) for high-stakes scenarios - Related to: Hierarchical Planning (5) with approval focus - Works with: Human-in-the-Loop (40) for approval - Complements: Workflow Agent (9) for execution - Used in: Web agents, robotic systems, enterprise automation

**References:** Planning literature; ACM tutorials on web agents; robotic planning; workflow systems

## **Pattern 42: Blackboard/Shared-Memory Pattern**

**Agent Type:** Agentic System

**What:** A coordination pattern where multiple loosely coupled agents read from and write to a centralized shared memory space (blackboard) and vector store, enabling asynchronous collaboration without direct agent-to-agent communication.

**Why:** Direct agent-to-agent communication creates tight coupling and complexity. Blackboard coordination provides simpler, more transparent collaboration that's easier to debug and monitor. This system-level infrastructure enables pragmatic multi-agent coordination.

**Mechanisms:** - Centralized shared memory/blackboard space - Task board with work items and status - Vector store for semantic information retrieval - Read/write protocols with locking mechanisms - Subscription and notification for changes - Event-driven agent activation - Conflict resolution for concurrent writes

**Agent Type Rationale:** Blackboard is classified as Agentic System because it provides system-level coordination infrastructure for multiple agents. The pattern focuses on shared state management and coordination rather than individual agent capabilities, representing a multi-agent orchestration framework.

**Related Patterns:** - Alternative to: Inter-Agent Communication (12) for simpler scenarios - Works with: Multi-Agent System (4) for coordination - Uses: Memory-Augmented (3) for shared storage - Complements: Orchestration (14) for workflow management - Related to: Monitoring/Observability (28) for state tracking

**References:** Classical blackboard architectures; modern LLM-augmented MAS; distributed shared memory systems

## **Pattern 43: Debate/Deliberation Pattern**

**Agent Type:** Agentic System

**What:** A multi-agent pattern where specialized agents engage in structured debate following propose-challenge-vote protocols to increase decision reliability and expose multiple perspectives on ambiguous or high-stakes decisions.

**Why:** Single agents can be biased or make errors on ambiguous tasks. Structured debate surfaces multiple viewpoints, adversarially tests proposals, and improves decision quality through collective intelligence. This system-level coordination creates emergent reliability.

**Mechanisms:** - Proposal generation by proposer agent(s) - Challenge and critique generation by critic agent(s) - Structured dialogue management and turn-taking - Voting or consensus mechanisms for resolution - Argument tracking and synthesis - User interface for human observation - Debate transcript recording for analysis

**Agent Type Rationale:** Debate/Deliberation is classified as Agentic System because it coordinates multiple agents in structured argumentation to achieve collective decision-making. The pattern provides system-level infrastructure for multi-perspective analysis rather than individual agent capabilities.

**Related Patterns:** - Specialized form of: Multi-Agent System (4) - Related to: Negotiation (21) but reliability-focused - Works with: Critic-Actor (8) for evaluation - Uses: Ensemble (35) for final voting - Complements: Explanation (22) for transparency - May include: Human-Agent Communication (13) for observation

**References:** ACM HCI papers on multi-agent dialogues; argumentation theory; debate protocols; adversarial collaboration

#### **Pattern 44: Composable DSLs / Contracts & Deontic Tokens**

**Agent Type:** Agentic System

**What:** A system-level pattern using domain-specific languages (DSLs) or structured contracts to express obligations, permissions, and prohibitions (deontic tokens) in forms that domain experts can author and that tooling can automatically validate and enforce at runtime.

**Why:** Natural language policies are ambiguous and unenforceable. Formal DSLs enable domain experts (clinicians, regulators, lawyers) to express constraints in their vocabulary while supporting automated verification, runtime enforcement, and compliance auditing. This system-level policy infrastructure ensures consistent enforcement across all agents.

**Mechanisms:** - DSL compilers and interpreters - Policy engines for rule evaluation - Contract-driven API gateways - Deontic token representation (burden, permit, embargo) - Automated policy verification and testing - Runtime policy enforcement - Policy-driven test suite generation

**Agent Type Rationale:** Composable DSLs is classified as Agentic System because it provides system-wide policy specification and enforcement infrastructure. The pattern enables consistent policy application across multiple agents, representing coordination-level governance beyond individual agent scope.

**Related Patterns:** - Extends: Inter-Agent Communication (12) with formal policies - Works with: Compliance/Governance (18) for enforcement - Complements: Constitutional AI (7) for value alignment - Used by: Access Control (19) for permissions - Enables: Audit Trail (20) for policy compliance tracking

**References:** Sepanosian & Milosevic (2025) “Towards a Toolchain for Formally Capturing and Monitoring Agent Accountability”; deontic logic; contract-driven development; policy-as-code

## Pattern 45: Hybrid Neuro-Symbolic Pattern

**Agent Type:** Agentic AI

**What:** An agent that combines statistical machine learning components (neural networks) with symbolic reasoning modules (rule engines, ontologies) to leverage strengths of both approaches for problems requiring both learning and explicit reasoning.

**Why:** Pure neural approaches lack explainability and struggle with constraints, while pure symbolic approaches can't learn from data. Hybrid systems combine adaptability with interpretability, particularly valuable in regulated domains (healthcare, legal) requiring both learning and explicit reasoning.

**Mechanisms:** - Pipeline integration (ML ↔ symbolic validation ↔ ML refinement) - Constraint injection into neural models - Ontology alignment with learned representations - Symbolic verification of neural outputs - Neuro-symbolic program synthesis - Rule extraction from neural networks - Constrained decoding with symbolic constraints

**Agent Type Rationale:** Hybrid Neuro-Symbolic is classified as Agentic AI because it demonstrates sophisticated autonomous reasoning combining learning with logical inference. The pattern exhibits genuine agency through its ability to both adapt from experience and apply explicit constraints—representing advanced cognitive capabilities.

**Related Patterns:** - Works with: Validation (27) for constraint checking - Complements: Explanation (22) for interpretability - Used in: Compliance/Governance (18) for rule adherence - Related to: Constitutional AI (7) for value constraints - Supports: Clinical and legal decision-making

**References:** Neuro-symbolic AI literature; constraint injection; hybrid reasoning systems; modular hybrid pattern taxonomies

## Pattern 46: Federated Privacy-Aware Pattern

**Agent Type:** Agentic System

**What:** A distributed system-level pattern enabling agents to train on local data at multiple sites while preserving privacy through techniques like federated learning, differential privacy, and secure multi-party computation.

**Why:** Sensitive data (medical records, financial data) often cannot leave its originating site due to regulations (HIPAA, GDPR) or privacy concerns. Federated approaches enable learning from distributed data while maintaining privacy, critical for healthcare and financial applications.

**Mechanisms:** - Federated learning with local training and aggregation - Differential privacy for privacy-preserving aggregation - Secure multi-party computation for sensitive operations - Client selection policies for participation - Model aggregation strategies (FedAvg, FedProx) - Privacy budget management - Audit and compliance for privacy requirements

**Agent Type Rationale:** Federated Privacy-Aware is classified as Agentic System because it provides system-level infrastructure for distributed, privacy-preserving multi-agent coordination. The pattern enables collaborative learning across organizational boundaries while maintaining privacy—a coordination capability transcending individual agents.

**Related Patterns:** - Enables: Multi-Agent System (4) across organizations - Required by: Compliance/Governance (18) for data privacy - Works with: Access Control (19) for data protection - Complements: Audit Trail (20) for privacy compliance - Used in: Healthcare, finance, cross-organizational AI

**References:** Federated learning literature; differential privacy; secure multi-party computation; privacy-preserving machine learning; medical AI systems

## Acknowledgments

This work was supported by UNSW Sydney, under a grant obtained by Professor Fethi Rabhi. The first author would like to thank Pieter van Schalkwyk (XMPRO Technologies) for many discussions on industrial applications and how the value of ODP-EL architecture and governance frameworks can support multi-agent environments. We also wish to thank Dr Basem Suleiman and Mr Chinmay Manchanda for their contributions to this project. Systematic documentation and structural organization of the pattern catalogue was conducted in collaboration with Claude (Anthropic). All conceptual frameworks, formal specifications, and domain expertise represent the work of the named authors.

## References and Further Reading

### Foundational Papers

**ReAct:** Yao et al. (2022) “ReAct: Synergizing Reasoning and Acting in Language Models”

**Tool-Using:** Schick et al. (2023) “Toolformer: Language Models Can Teach Themselves to Use Tools”

**Memory-Augmented:** - Weng (2023) “LLM Powered Autonomous Agents” - Packer et al. (2023) “MemGPT”

**Multi-Agent Systems:** - Stone & Veloso (2000) “Multiagent Systems: A Survey” - Wu et al. (2023) “AutoGen”

**Hierarchical Planning:** - Ahn et al. (2022) “Do As I Can, Not As I Say” - Huang et al. (2022) “Language Models as Zero-Shot Planners”

**Reflexion:** Shinn et al. (2023) “Reflexion: Language Agents with Verbal Reinforcement Learning”

**Constitutional AI:** Bai et al. (2022) “Constitutional AI: Harmlessness from AI Feedback”

**Communication Theory:** - Searle (1969) “Speech Acts: An Essay in the Philosophy of Language” - Austin (1962) “How to Do Things with Words” - Wooldridge (2009) “An Introduction to MultiAgent Systems”

**ODP Enterprise Language:** - ISO/IEC 15414 “ODP Enterprise Language” - Linington et al. (2011) “Building Enterprise Systems with ODP” - FIPA (2002) “FIPA Communicative Act Library Specification”

### Domain Applications

**Healthcare AI:** - Burgos & Milosevic (2025) “Consumer-Centered Selection of Relevant Clinical Trials Using Agent AI” - HL7 FHIR Specification

**Enterprise Systems:** - Sepanosian & Milosevic (2025) “Towards a Toolchain for Formally Capturing and Monitoring Agent Accountability”

### Design Pattern Literature

**Classic Patterns:** - Gamma et al. (1994) “Design Patterns: Elements of Reusable Object-Oriented Software” - Buschmann et al. (1996) “Pattern-Oriented Software Architecture”

**Agent Patterns:** - Aridor & Lange (1998) “Agent Design Patterns” - Oluyomi et al. (2007) “A Goal-Oriented Approach for Composing Agent Design Patterns”
